# Supplementary material for: SparseLNR: Accelerating Sparse Tensor Computations Using Loop Nest Restructuring
Source: arXiv:2205.11622 source file (2022-05-23)
Supplement: Supplementary file 1 [file additional.tex]

% Evaluation graph 4 graphs in a row

\begin{figure*}[ht]
    \centering
    \begin{subfigure}[t]{0.25\textwidth}
        \centering
        \includegraphics[width=1\linewidth]{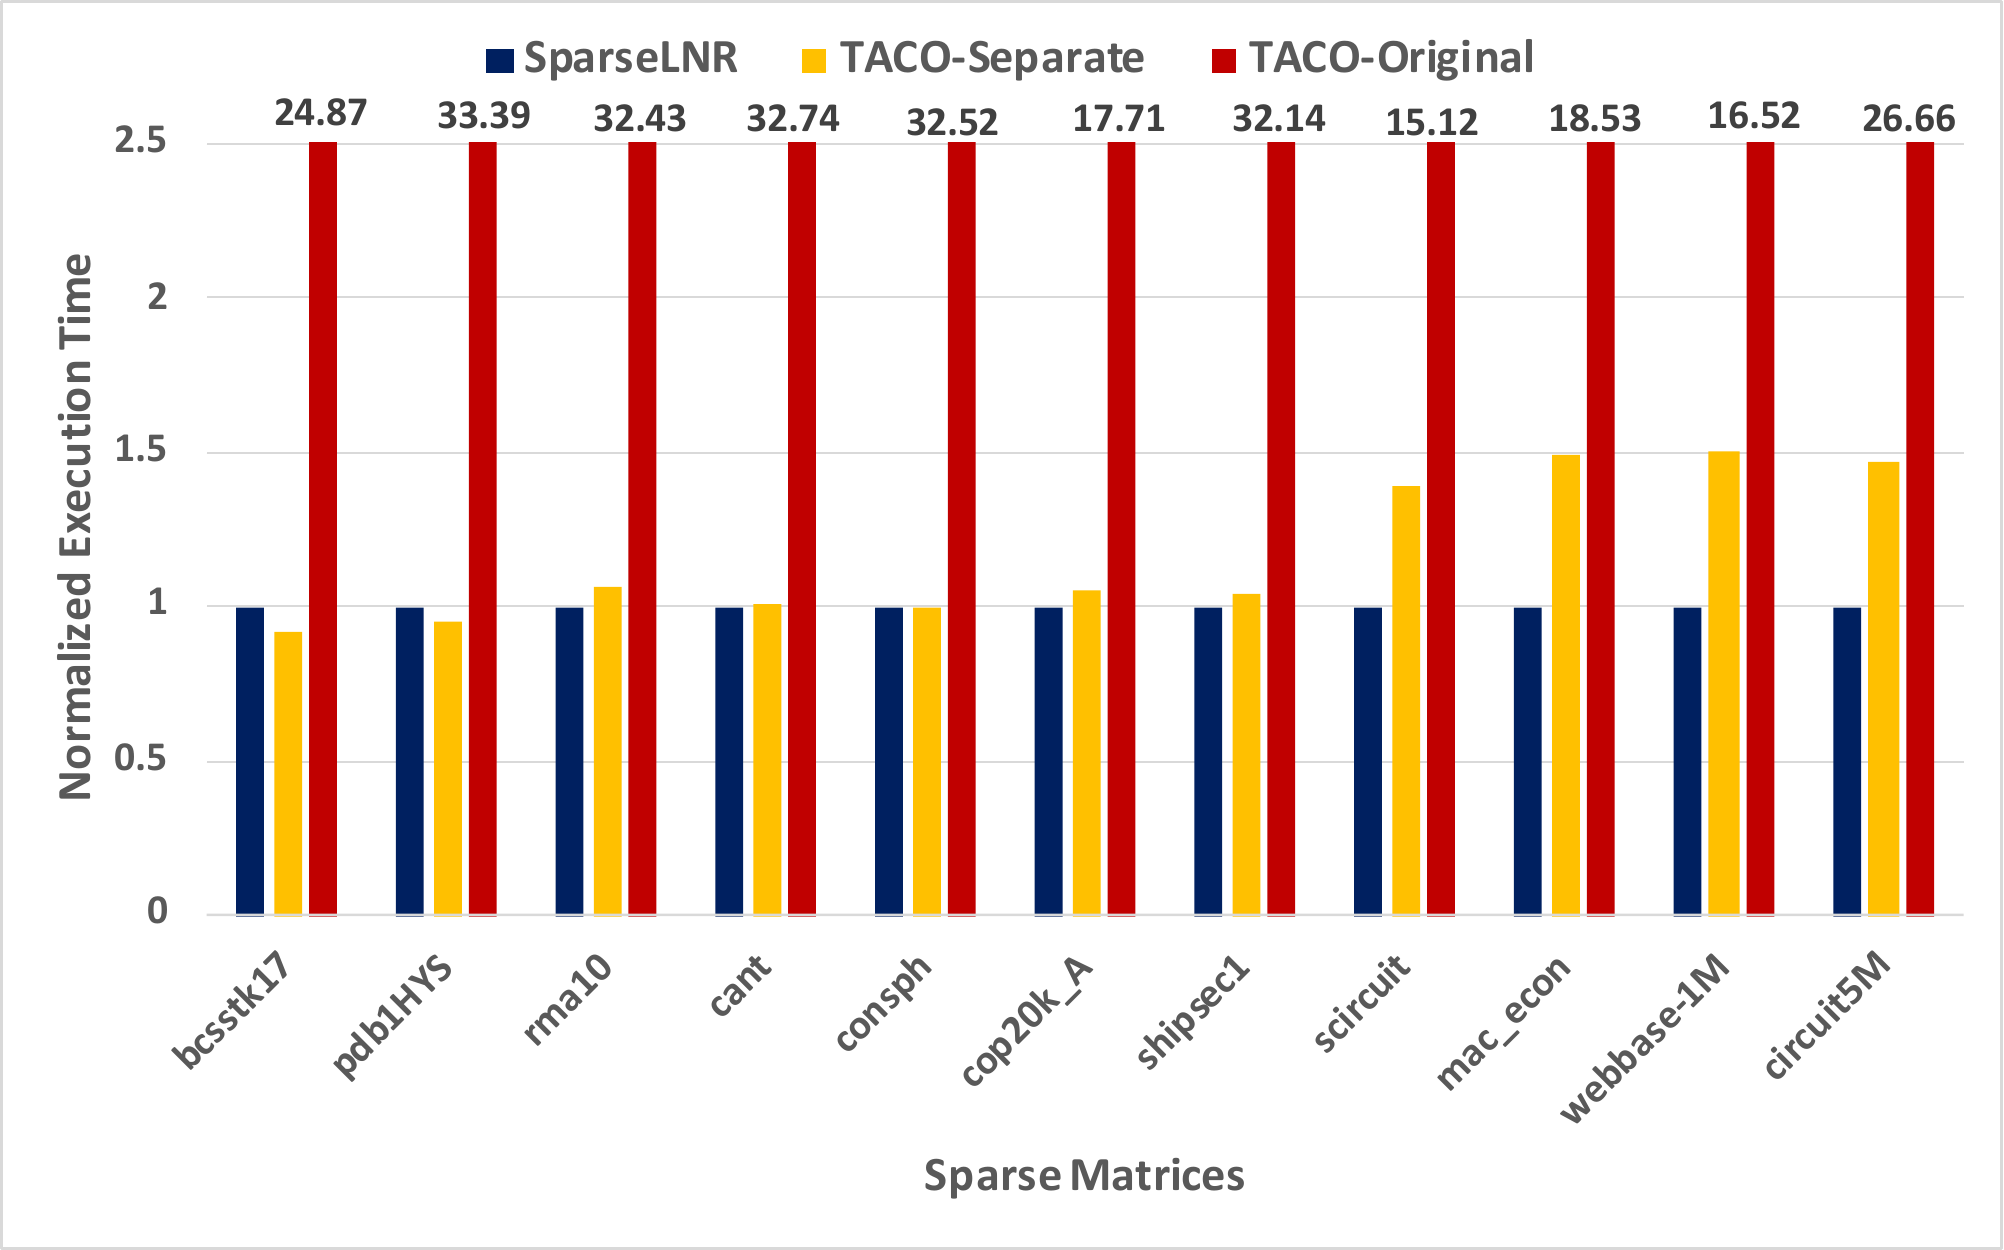}
        \vspace{-10pt}
        \caption{<SDDMM, SpMM> single-thread}
        \vspace{-10pt}
        \label{fig:sddmm-spmm-single-thread}
        \Description[sddmm-spmm original iteration graph]{<long description>}
    \end{subfigure}%
    \hfill
    \begin{subfigure}[t]{0.25\textwidth}
        \centering
        \includegraphics[width=1\linewidth]{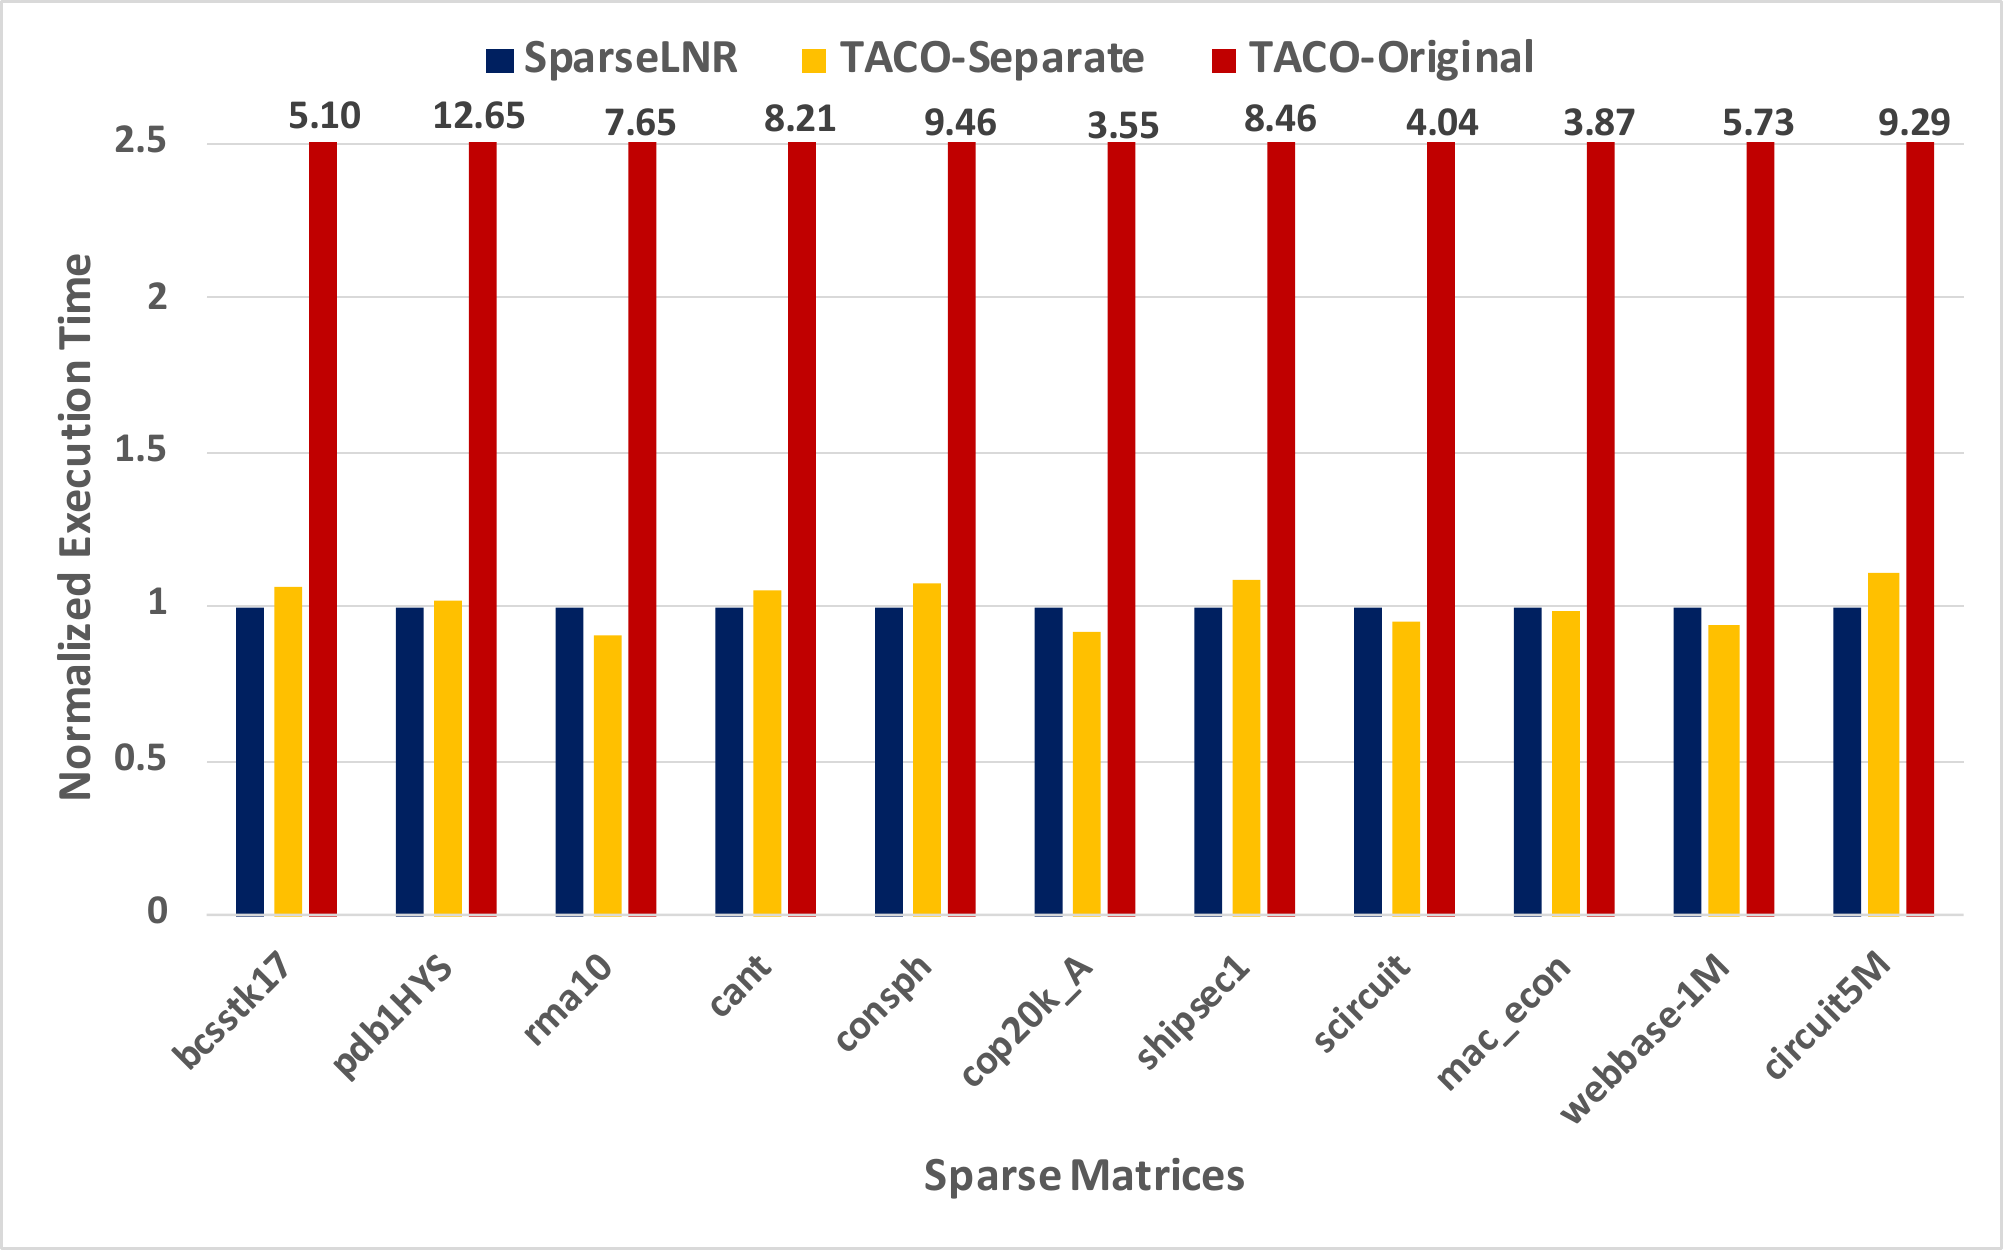}
        \vspace{-10pt}
        \caption{<SDDMM, SPMM> multi-threads}
        \vspace{-10pt}
        \label{fig:sddmm-spmm-multi-thread}
        \Description[sddmm-spmm original iteration graph]{<long description>}
    \end{subfigure}%
    \hfill%
    \begin{subfigure}[t]{0.25\textwidth}
        \centering
        \includegraphics[width=1\linewidth]{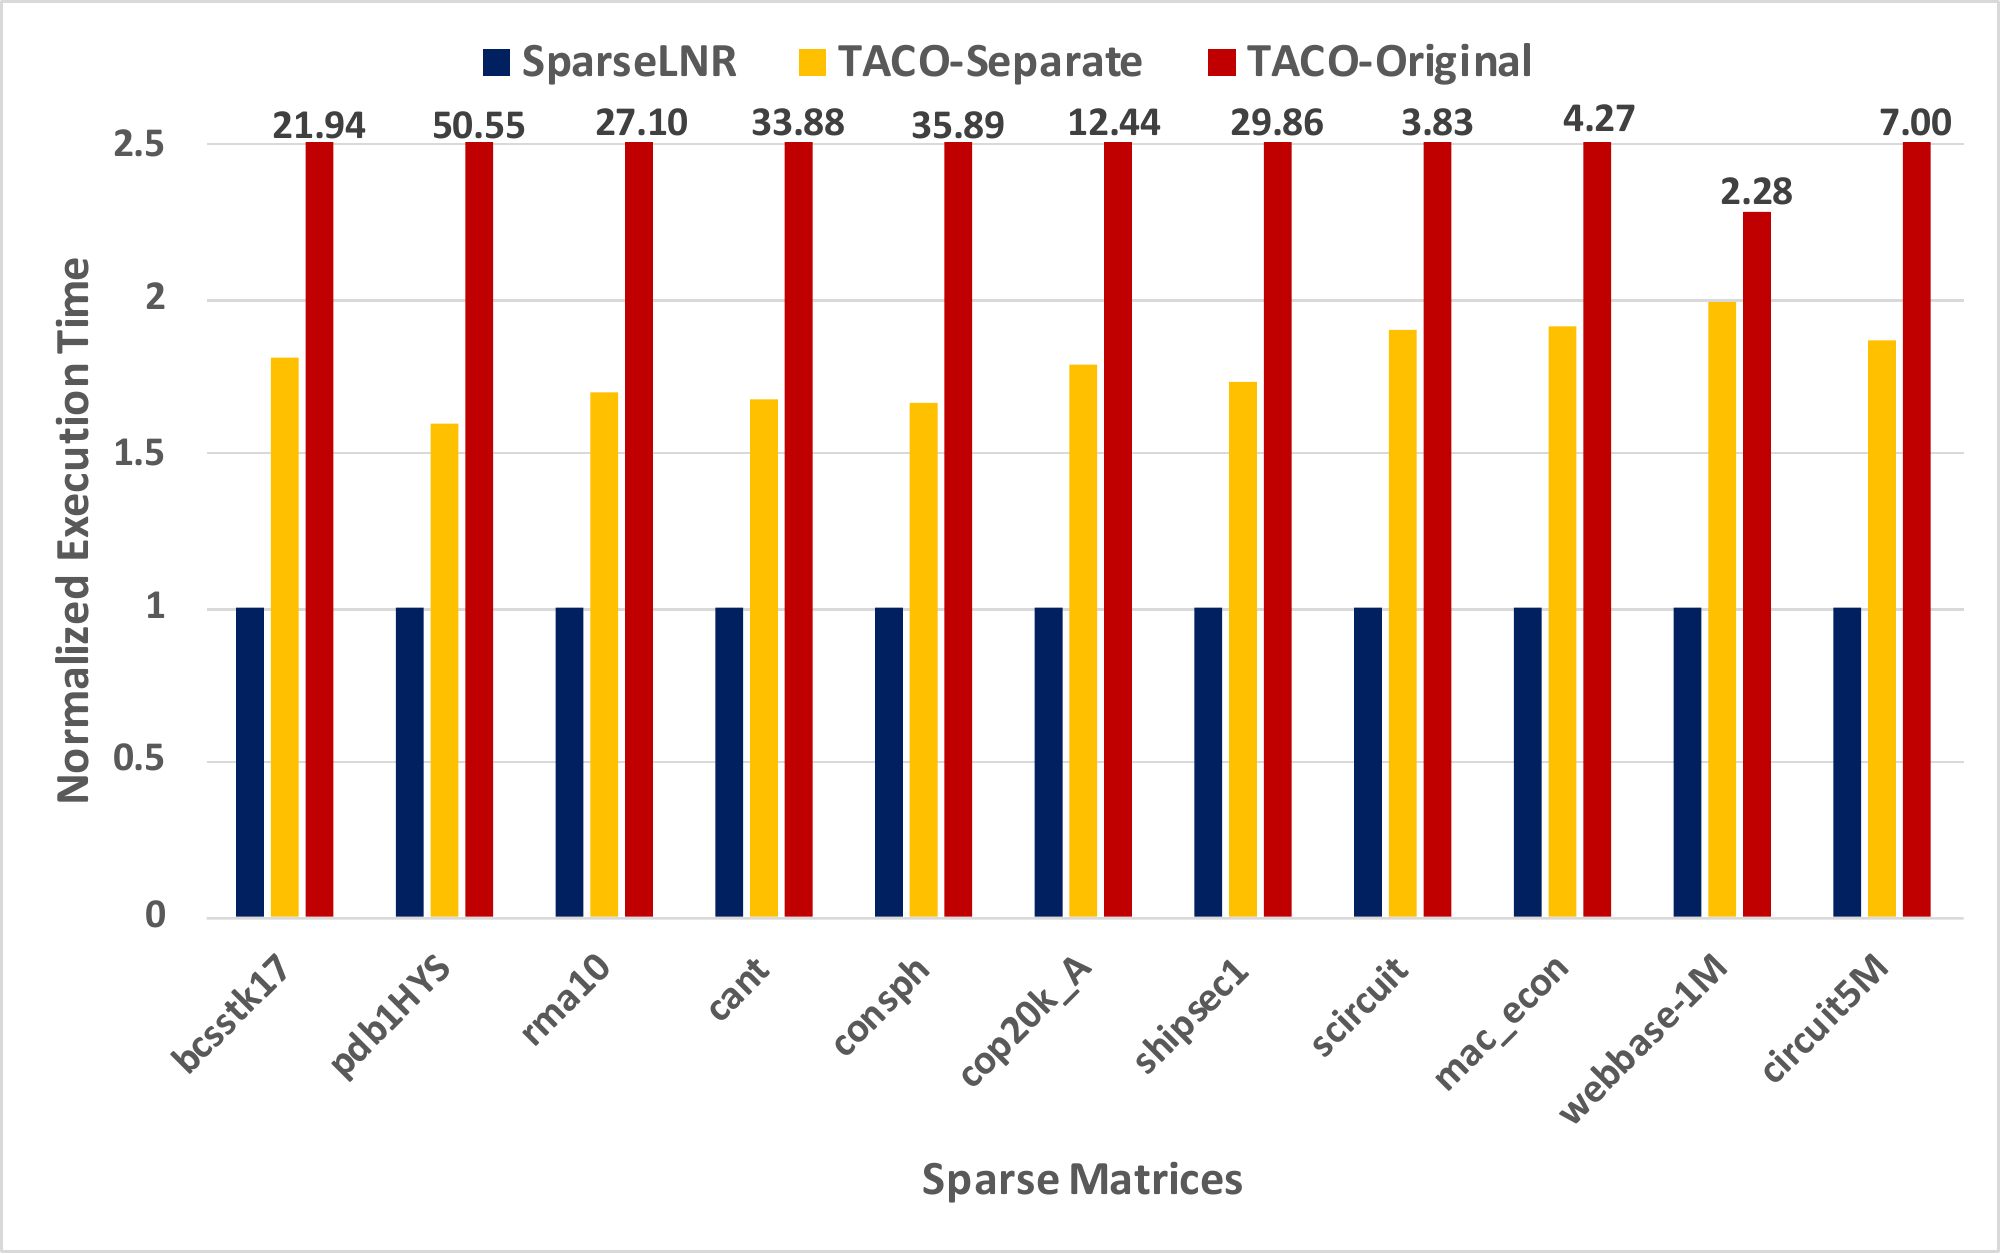}
        \vspace{-10pt}
        \caption{<SpMMH, GeMM> single-thread}
        \vspace{-10pt}
        \label{fig:spgemmh-gemm-single-thread}
        \Description[sddmm-spmm original iteration graph]{<long description>}
    \end{subfigure}%
    \hfill
    \begin{subfigure}[t]{0.25\textwidth}
        \centering
        \includegraphics[width=1\linewidth]{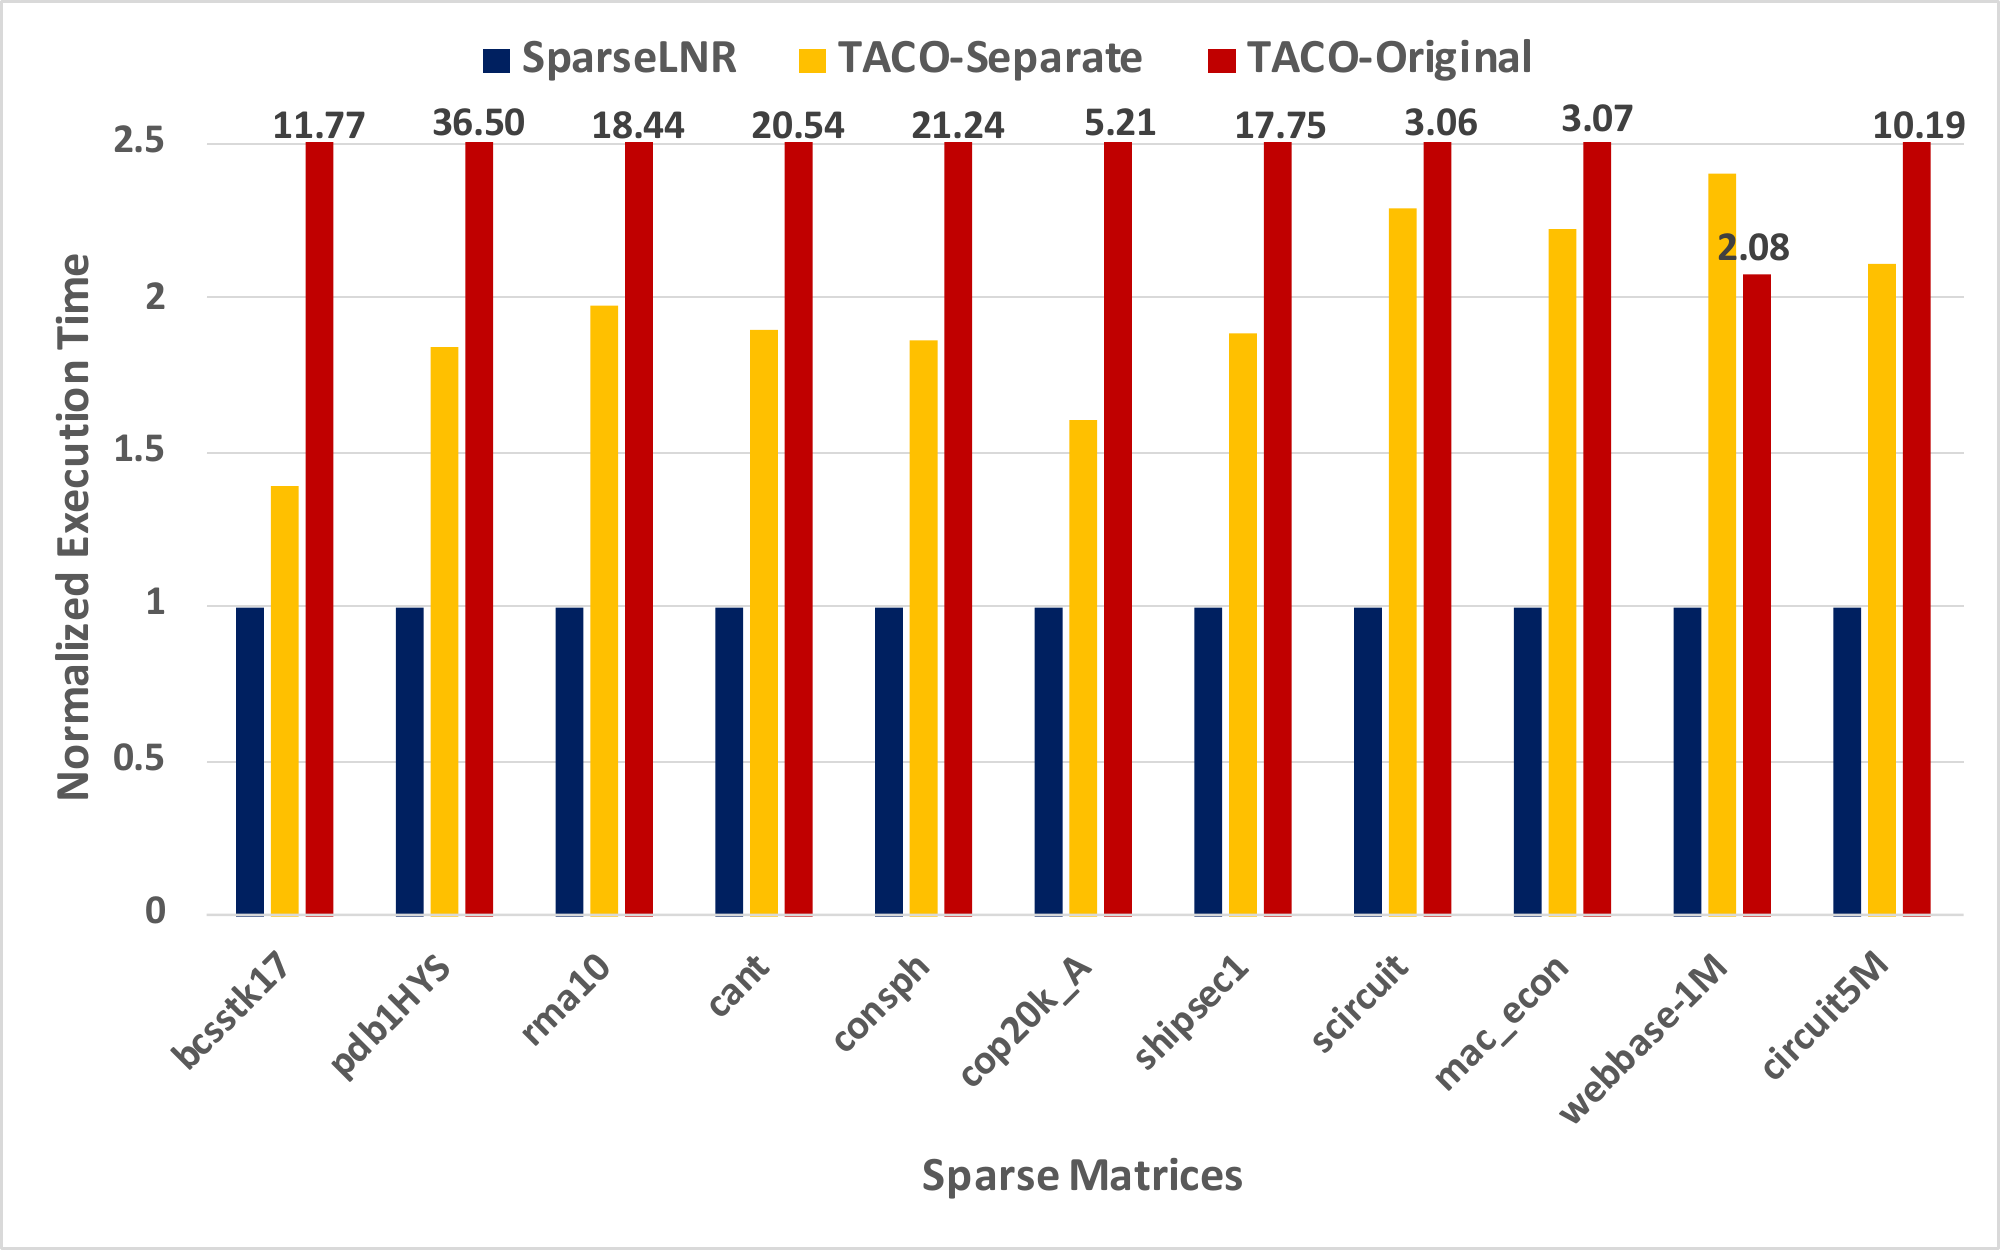}
        \vspace{-10pt}
        \caption{<SpMMH, GeMM> single-thread}
        \vspace{-10pt}
        \label{fig:spgemmh-gemm-multi-thread}
        \Description[sddmm-spmm original iteration graph]{<long description>}
    \end{subfigure}%
    \vskip\baselineskip
    \begin{subfigure}[t]{0.25\textwidth}
        \centering
        \includegraphics[width=1\linewidth]{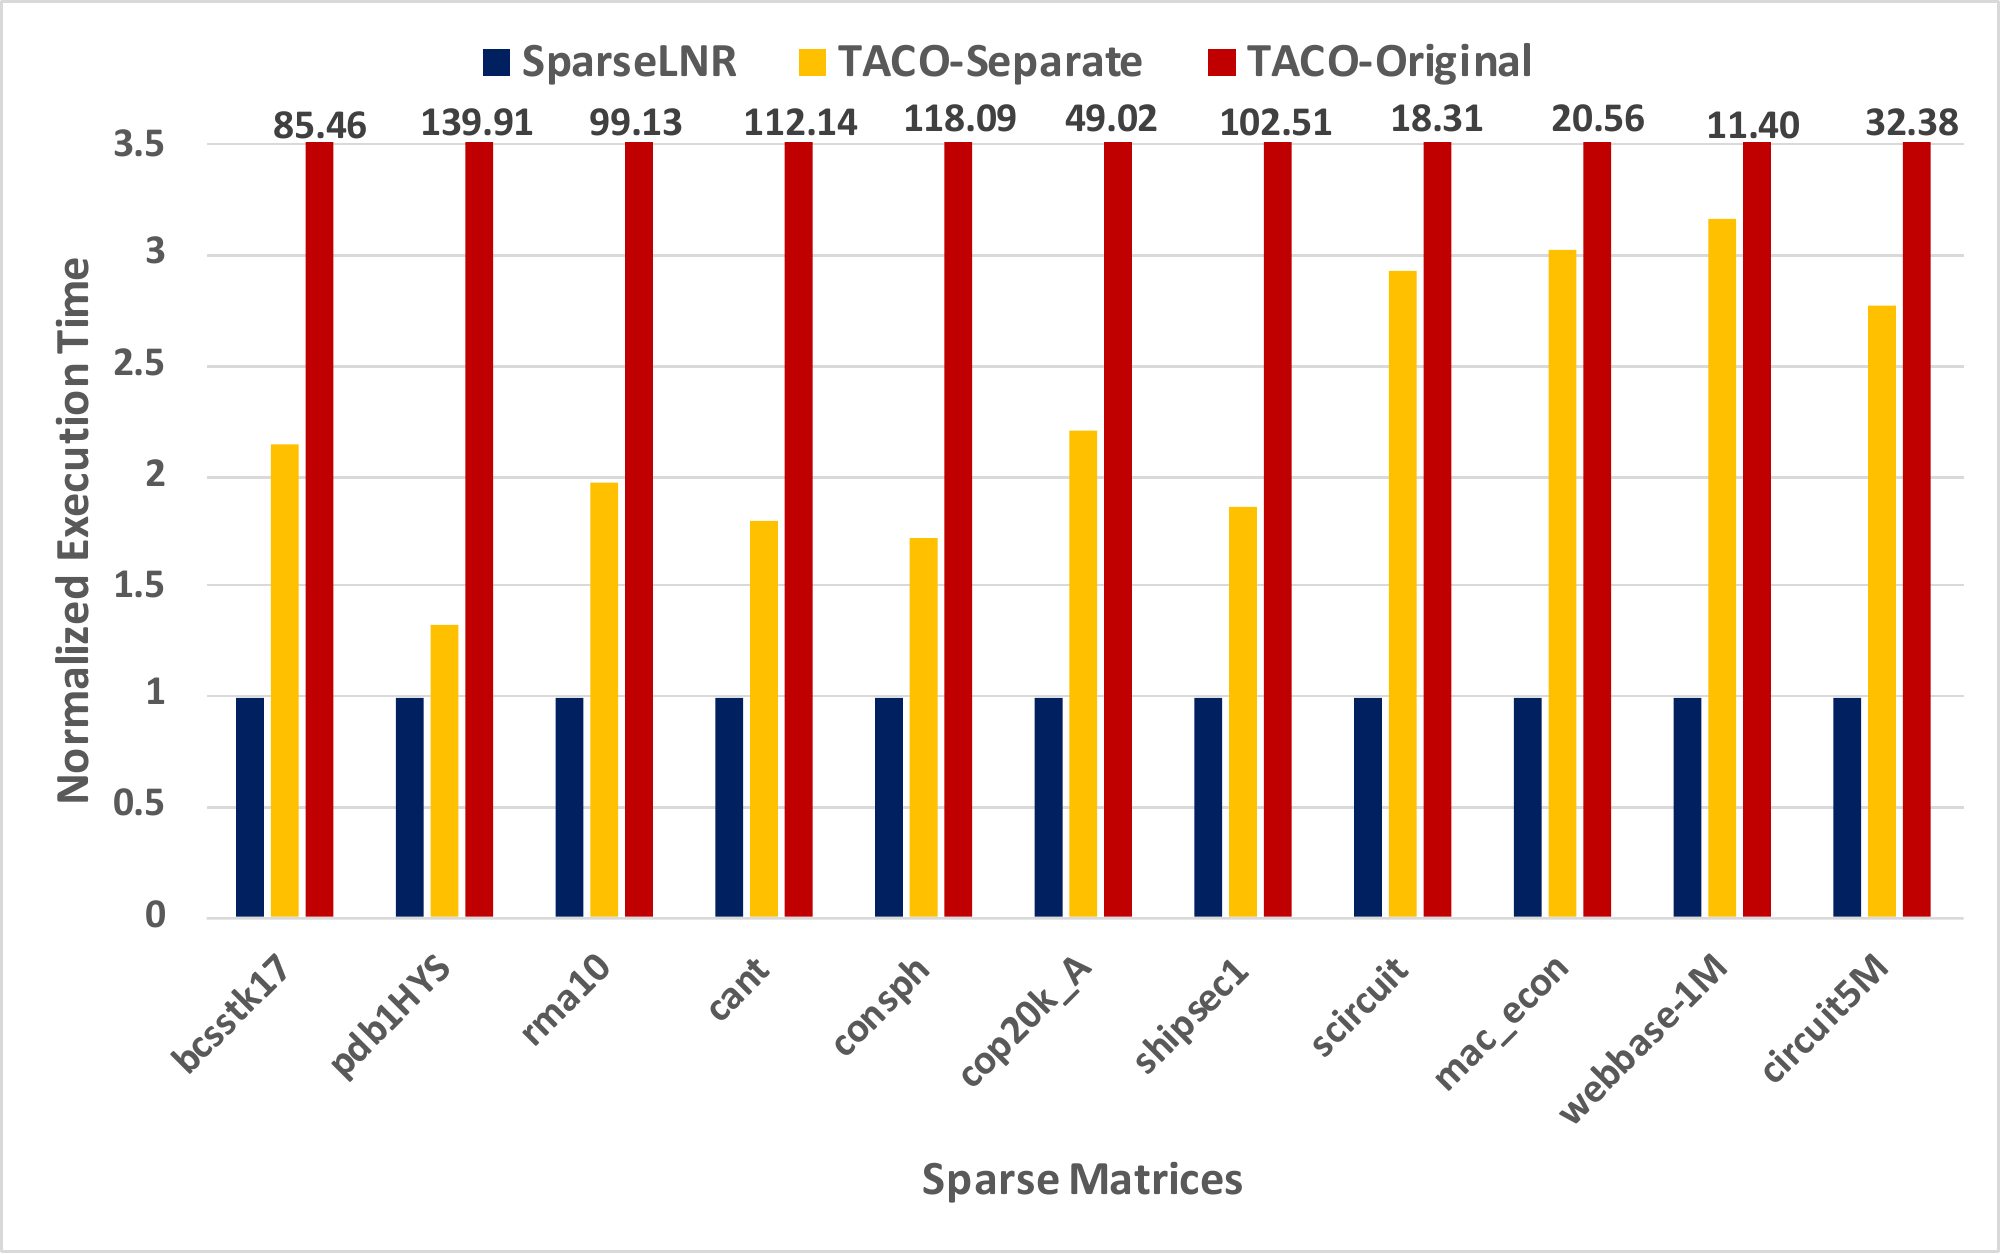}
        \vspace{-10pt}
        \caption{<SpMM, GeMM> single-thread}
        \vspace{-10pt}
        \label{fig:spmm-gemm-single-thread}
        \Description[sddmm-spmm original iteration graph]{<long description>}
    \end{subfigure}%
    \hfill
    \begin{subfigure}[t]{0.25\textwidth}
        \centering
        \includegraphics[width=1\linewidth]{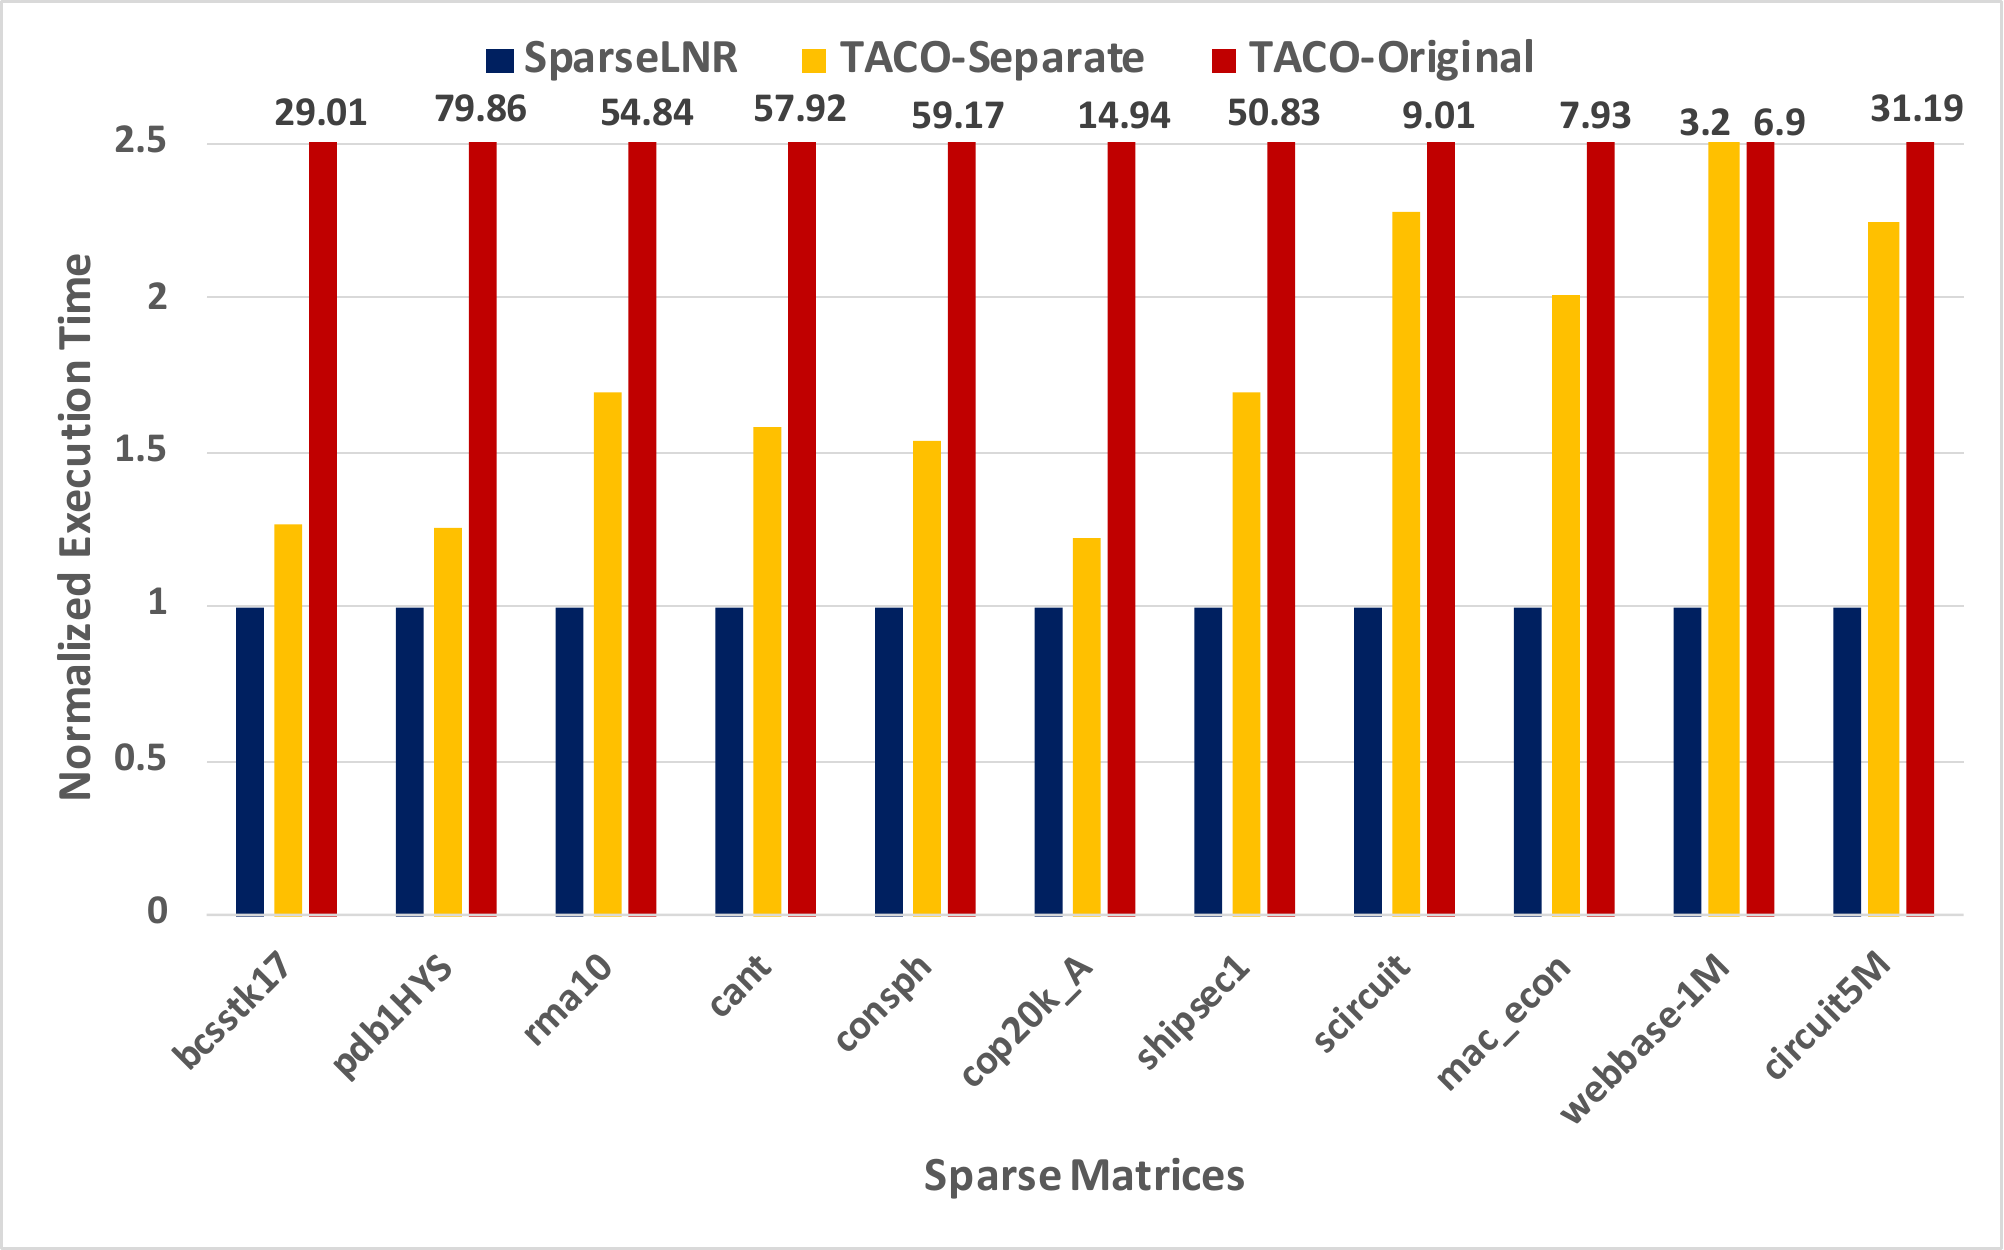}
        \vspace{-10pt}
        \caption{<SpMM, GeMM> multi-threads}
        \vspace{-10pt}
        \label{fig:spmm-gemm-multi-thread}
        \Description[sddmm-spmm original iteration graph]{<long description>}
    \end{subfigure}%
    \hfill%
    \begin{subfigure}[t]{0.25\textwidth}
        \centering
        \includegraphics[width=1\linewidth]{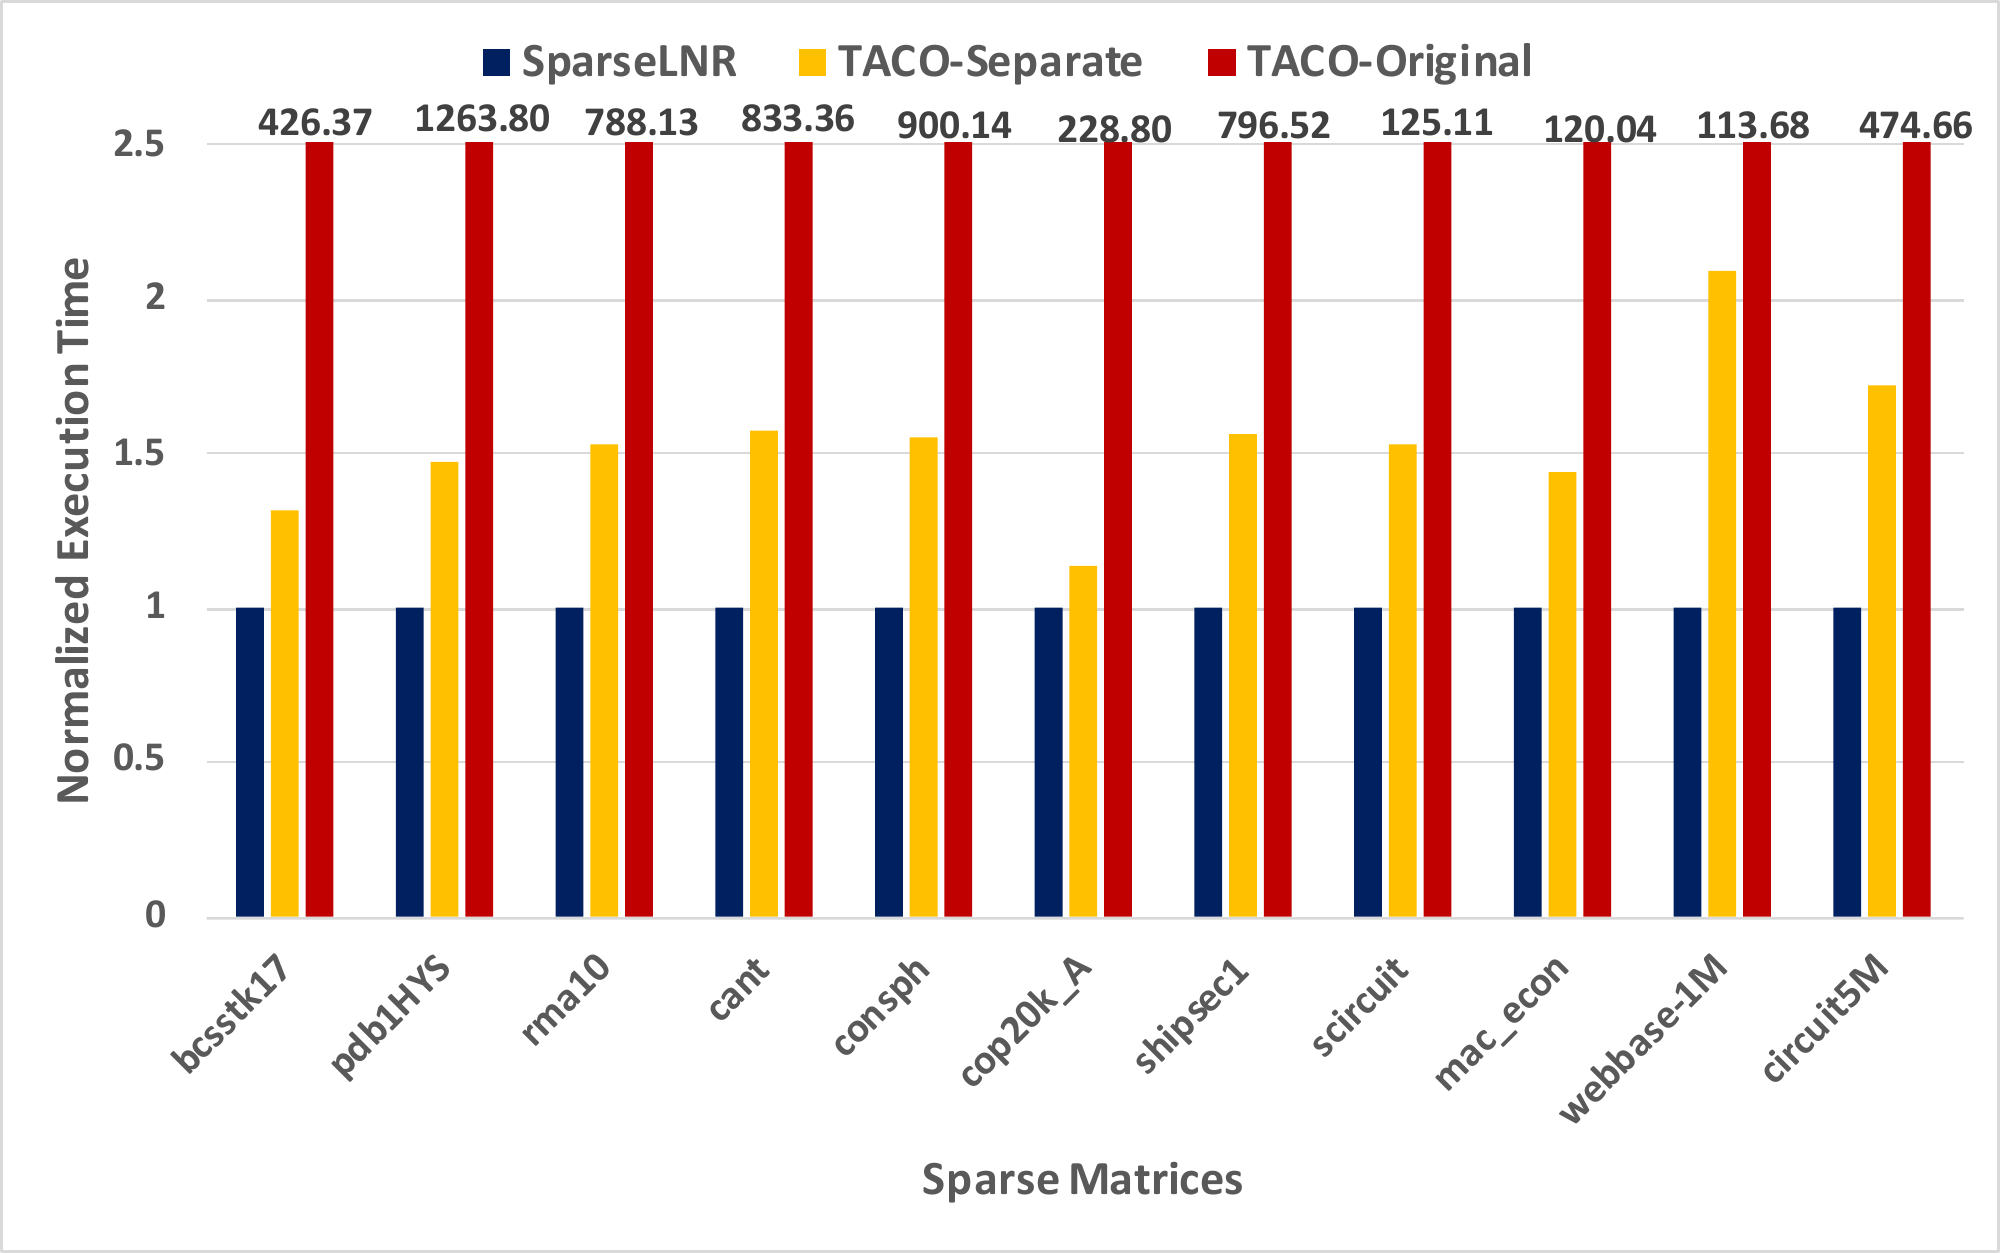}
        \vspace{-10pt}
        \caption{<SDDMM, SpMM, GeMM> single-thread}
        \vspace{-10pt}
        \label{fig:sddmm-spmm-gemm-single-thread}
        \Description[sddmm-spmm original iteration graph]{<long description>}
    \end{subfigure}%
    \hfill%
    \begin{subfigure}[t]{0.25\textwidth}
        \centering
        \includegraphics[width=1\linewidth]{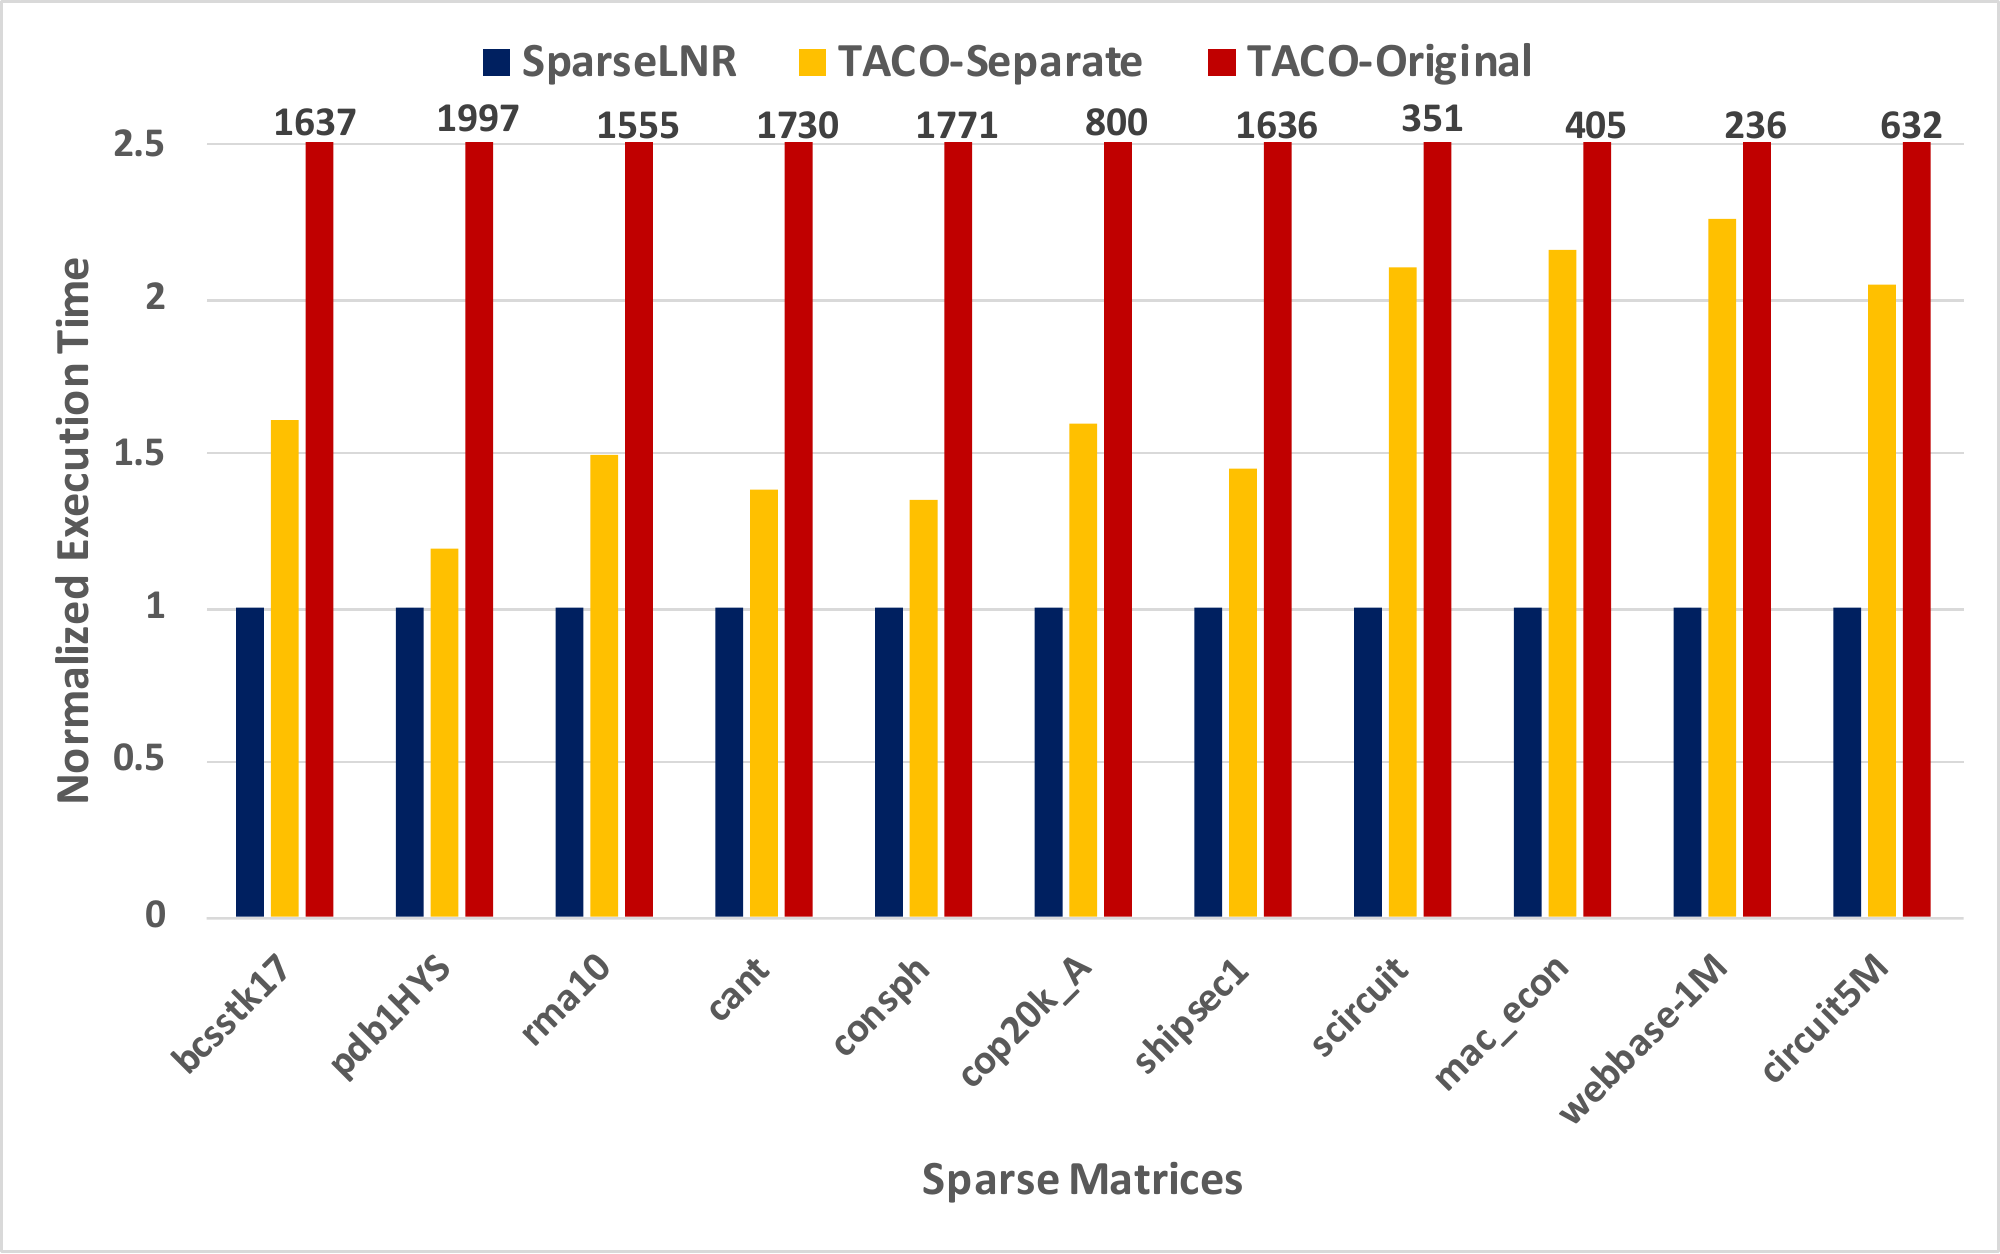}
        \vspace{-10pt}
        \caption{<SDDMM, SpMM, GeMM> multi-threads}
        \vspace{-10pt}
        \label{fig:sddmm-spmm-gemm-multi-thread}
        \Description[sddmm-spmm original iteration graph]{<long description>}
    \end{subfigure}%
    \vskip\baselineskip
    \begin{subfigure}[t]{0.25\textwidth}
        \centering
        \includegraphics[width=1\linewidth]{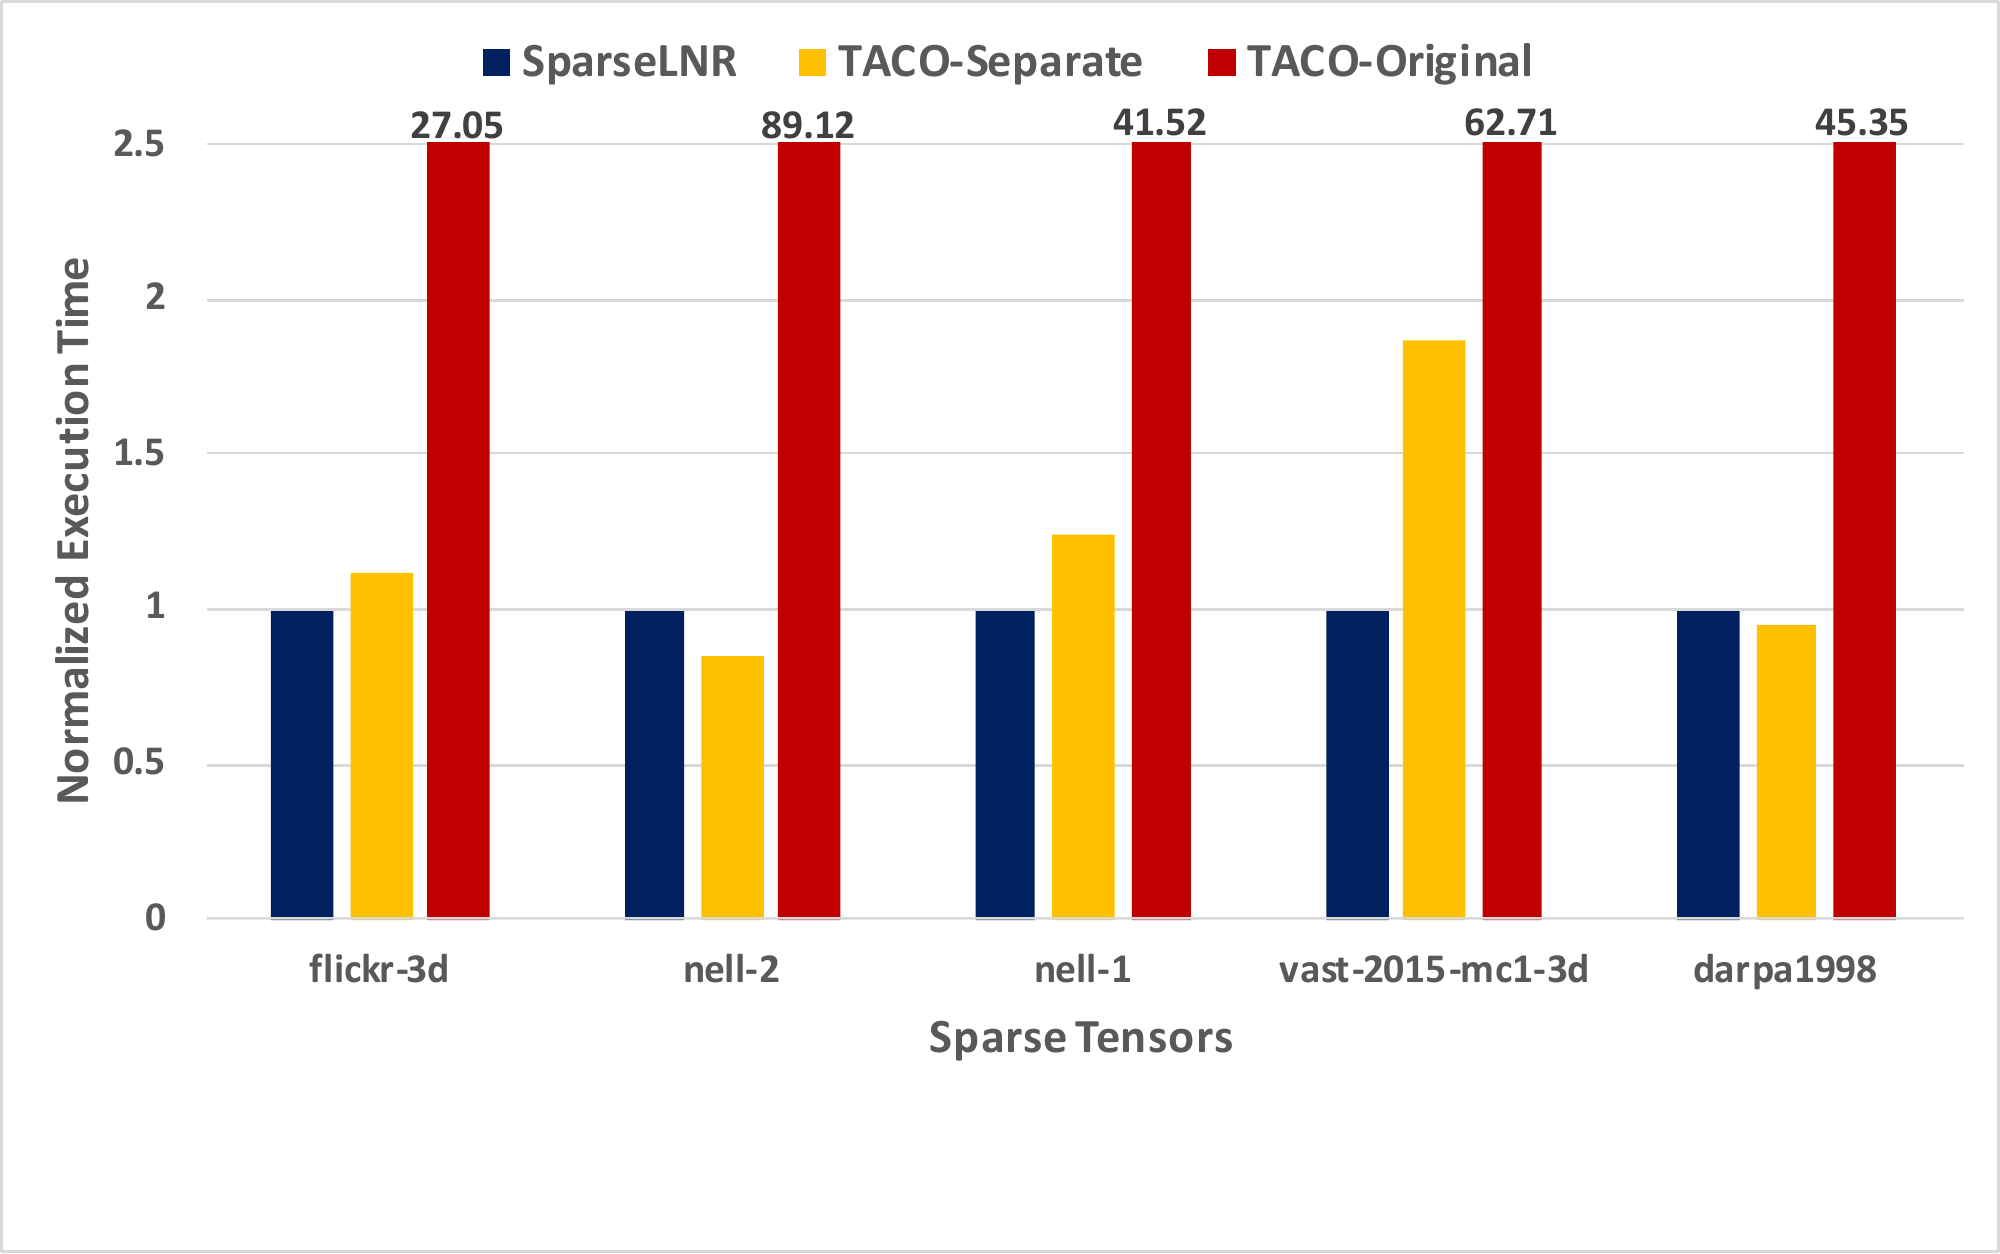}
        \vspace{-10pt}
        \caption{<MTTKRP, GeMM> single-thread}
        \vspace{-10pt}
        \label{fig:mttkrp-gemm-single-thread}
        \Description[sddmm-spmm original iteration graph]{<long description>}
    \end{subfigure}%
    \hfill
    \begin{subfigure}[t]{0.24\textwidth}
        \centering
        \includegraphics[width=1\linewidth]{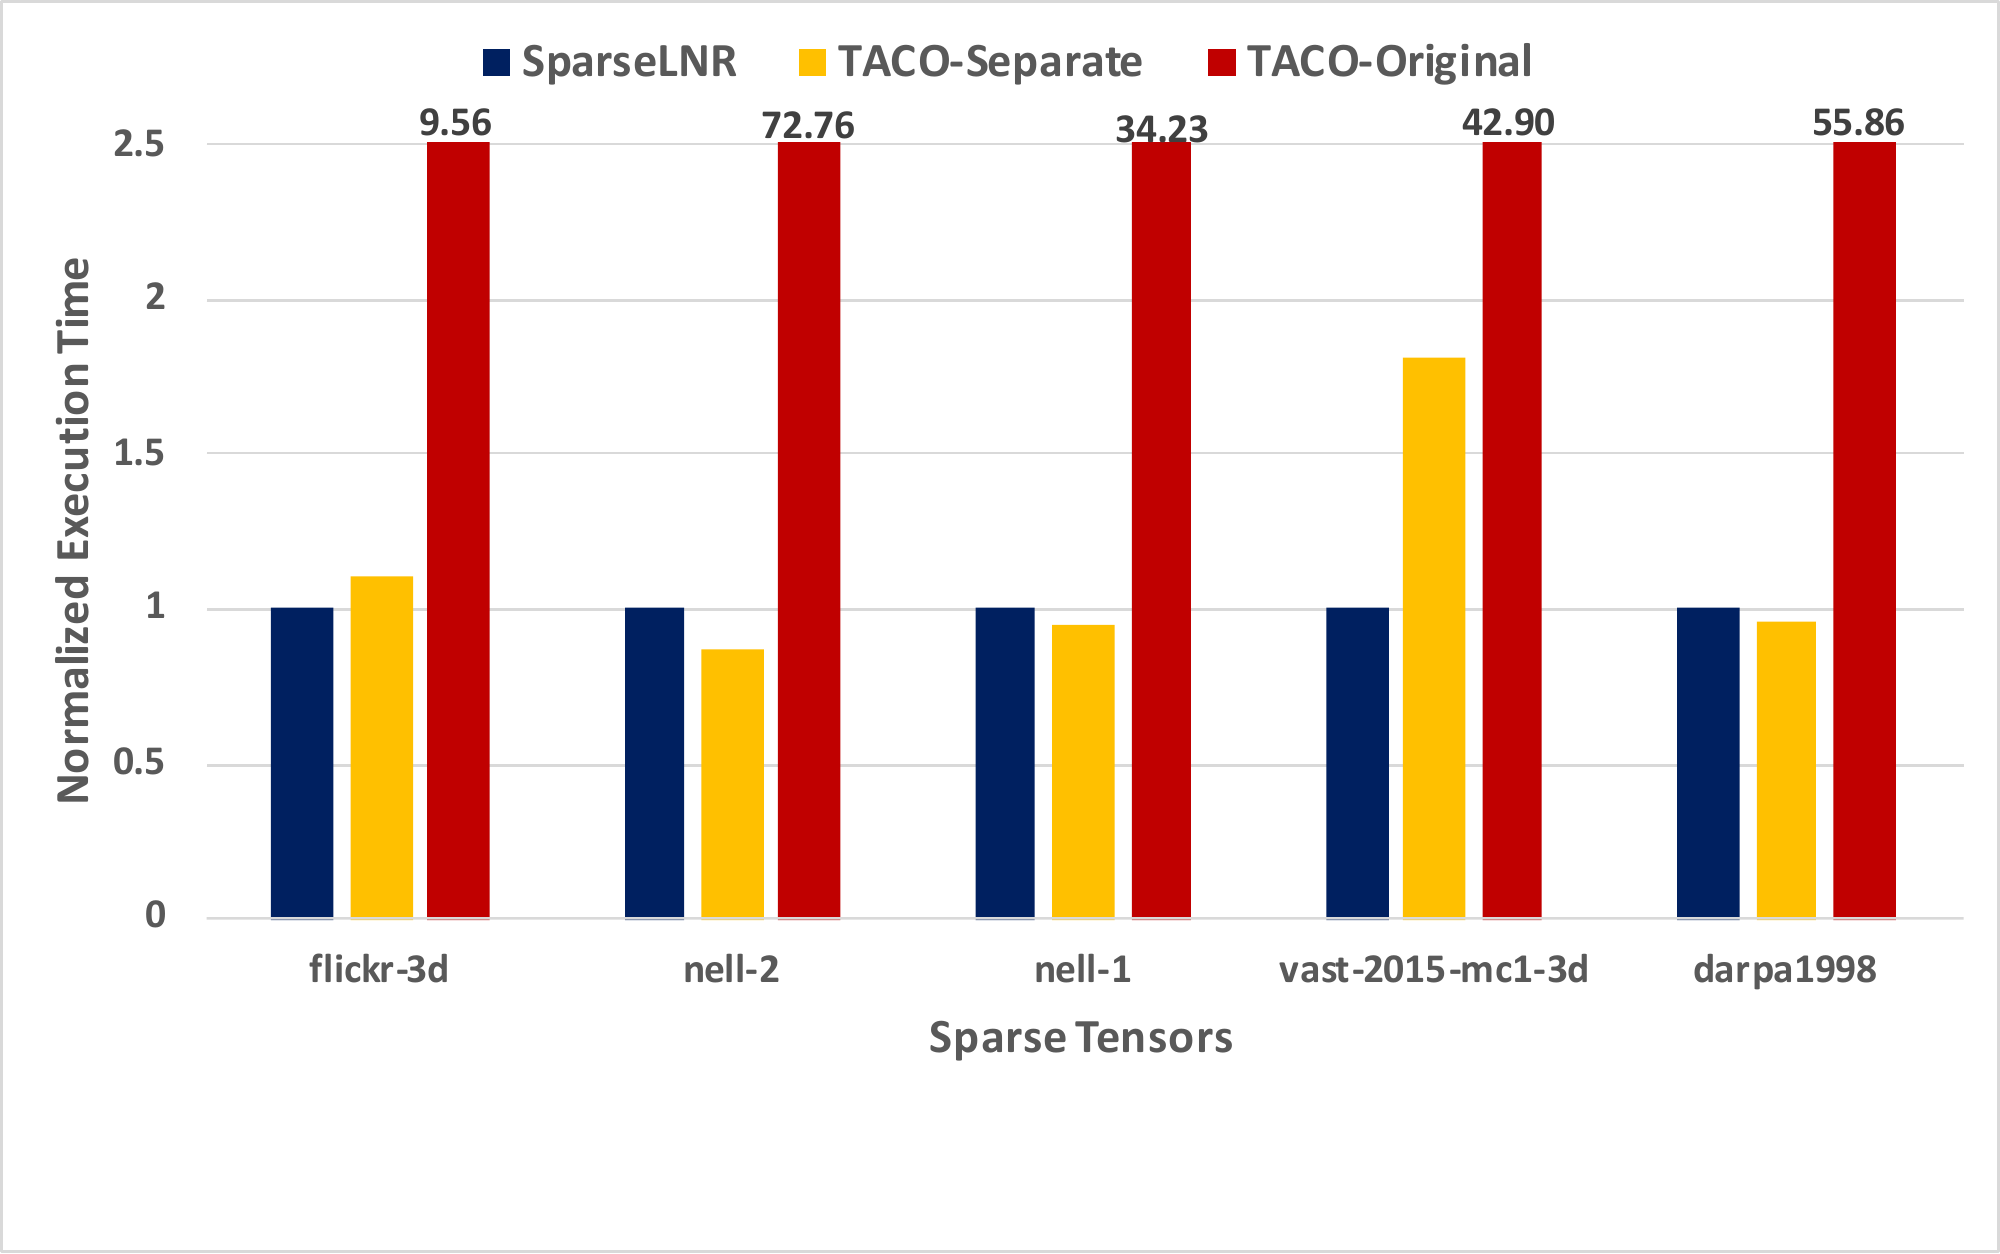}
        \vspace{-10pt}
        \caption{<MTTKRP, GeMM> multi-threads}
        \vspace{-10pt}
        \label{fig:mttkrp-gemm-multi-thread}
        \Description[sddmm-spmm original iteration graph]{<long description>}
    \end{subfigure}%
    \hfill%
    \begin{subfigure}[t]{0.24\textwidth}
        \centering
        \includegraphics[width=1\linewidth]{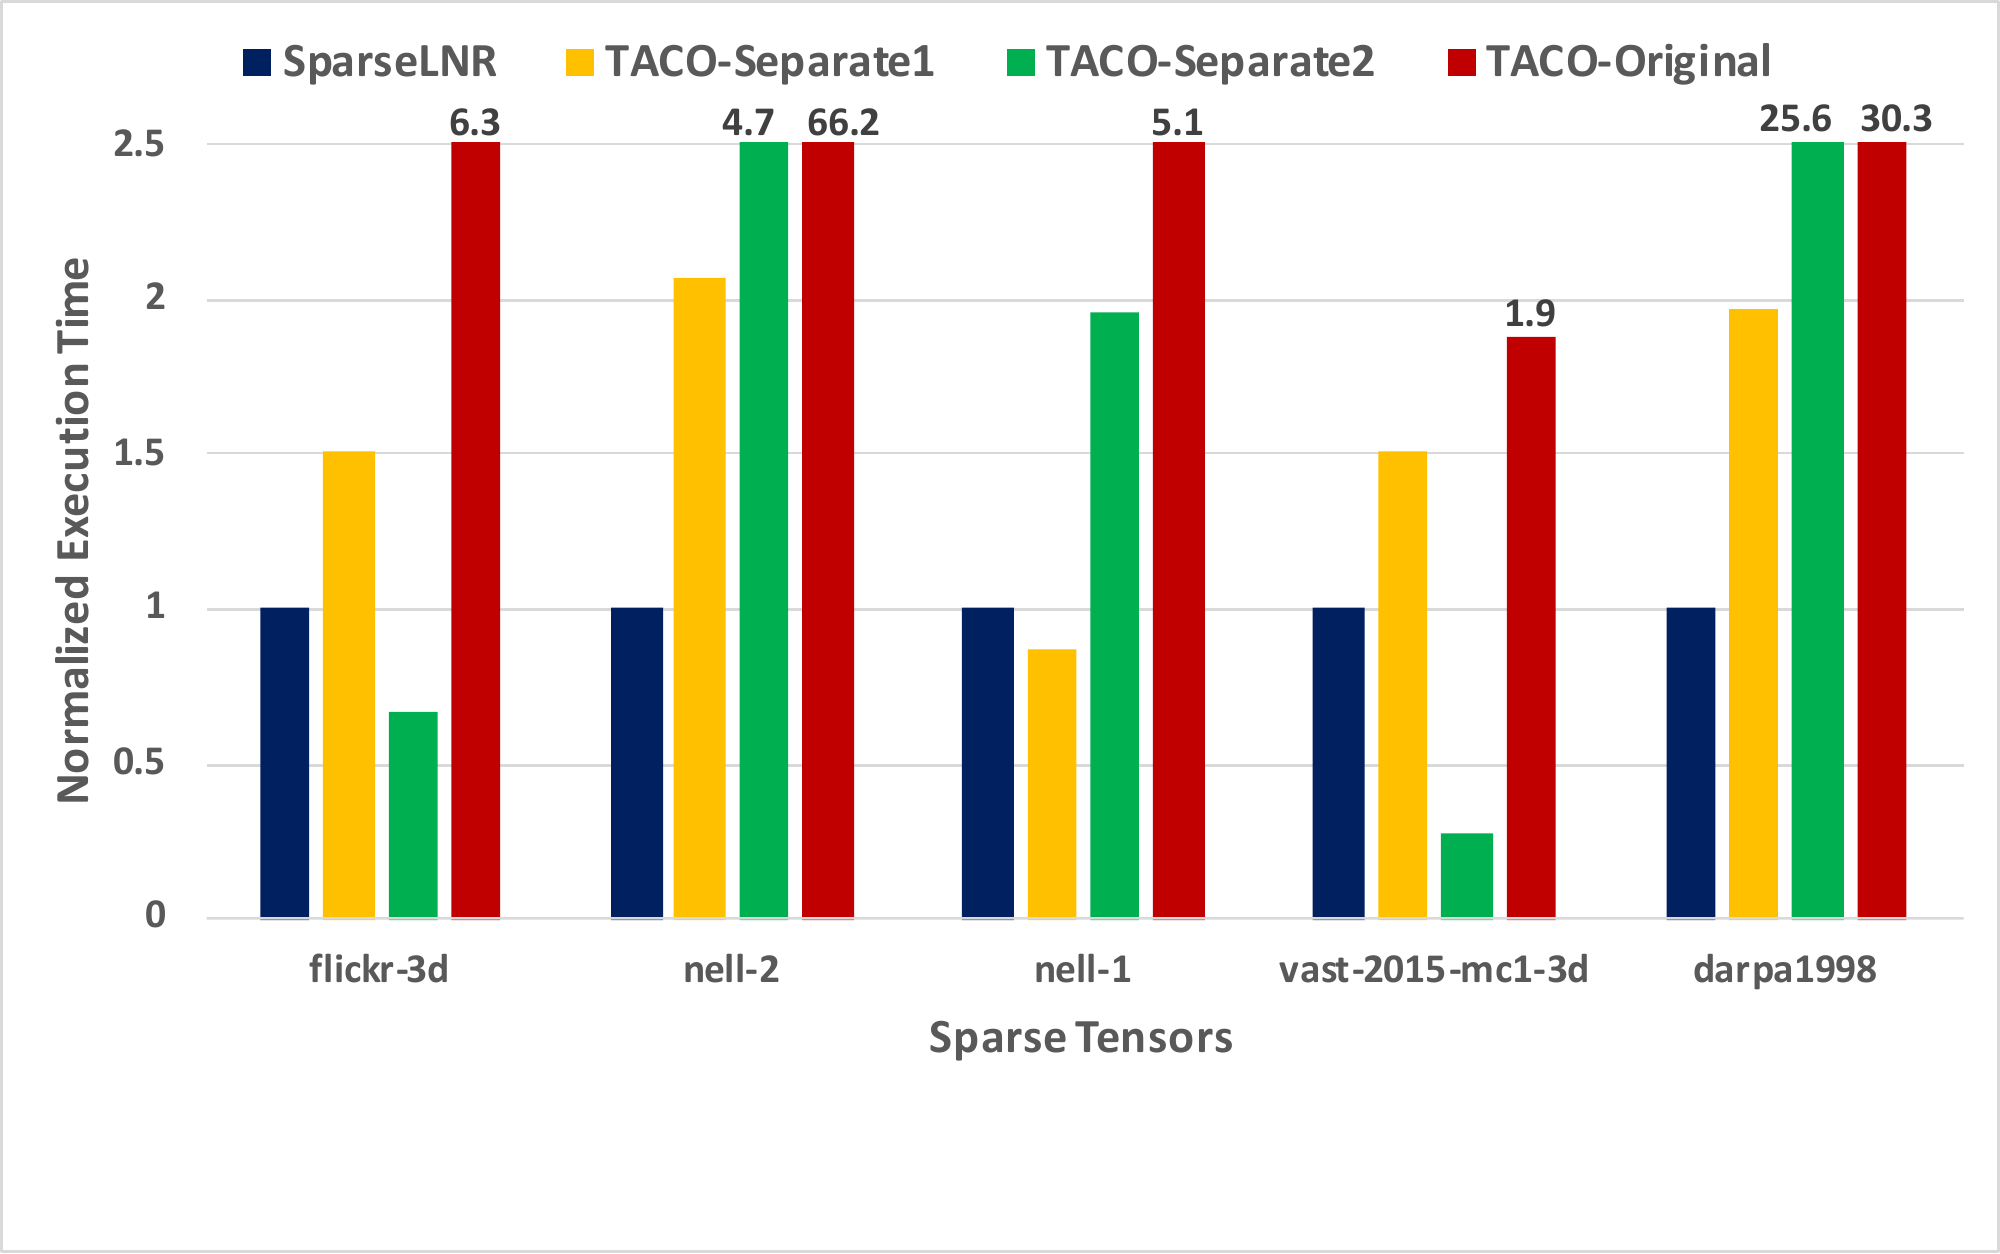}
        \vspace{-10pt}
        \caption{<SpTTM, SpTTM> single-thread}
        \vspace{-10pt}
        \label{fig:ttm-ttm-single-thread}
        \Description[sddmm-spmm original iteration graph]{<long description>}
    \end{subfigure}%
    \hfill%
    \begin{subfigure}[t]{0.24\textwidth}
        \centering
        \includegraphics[width=1\linewidth]{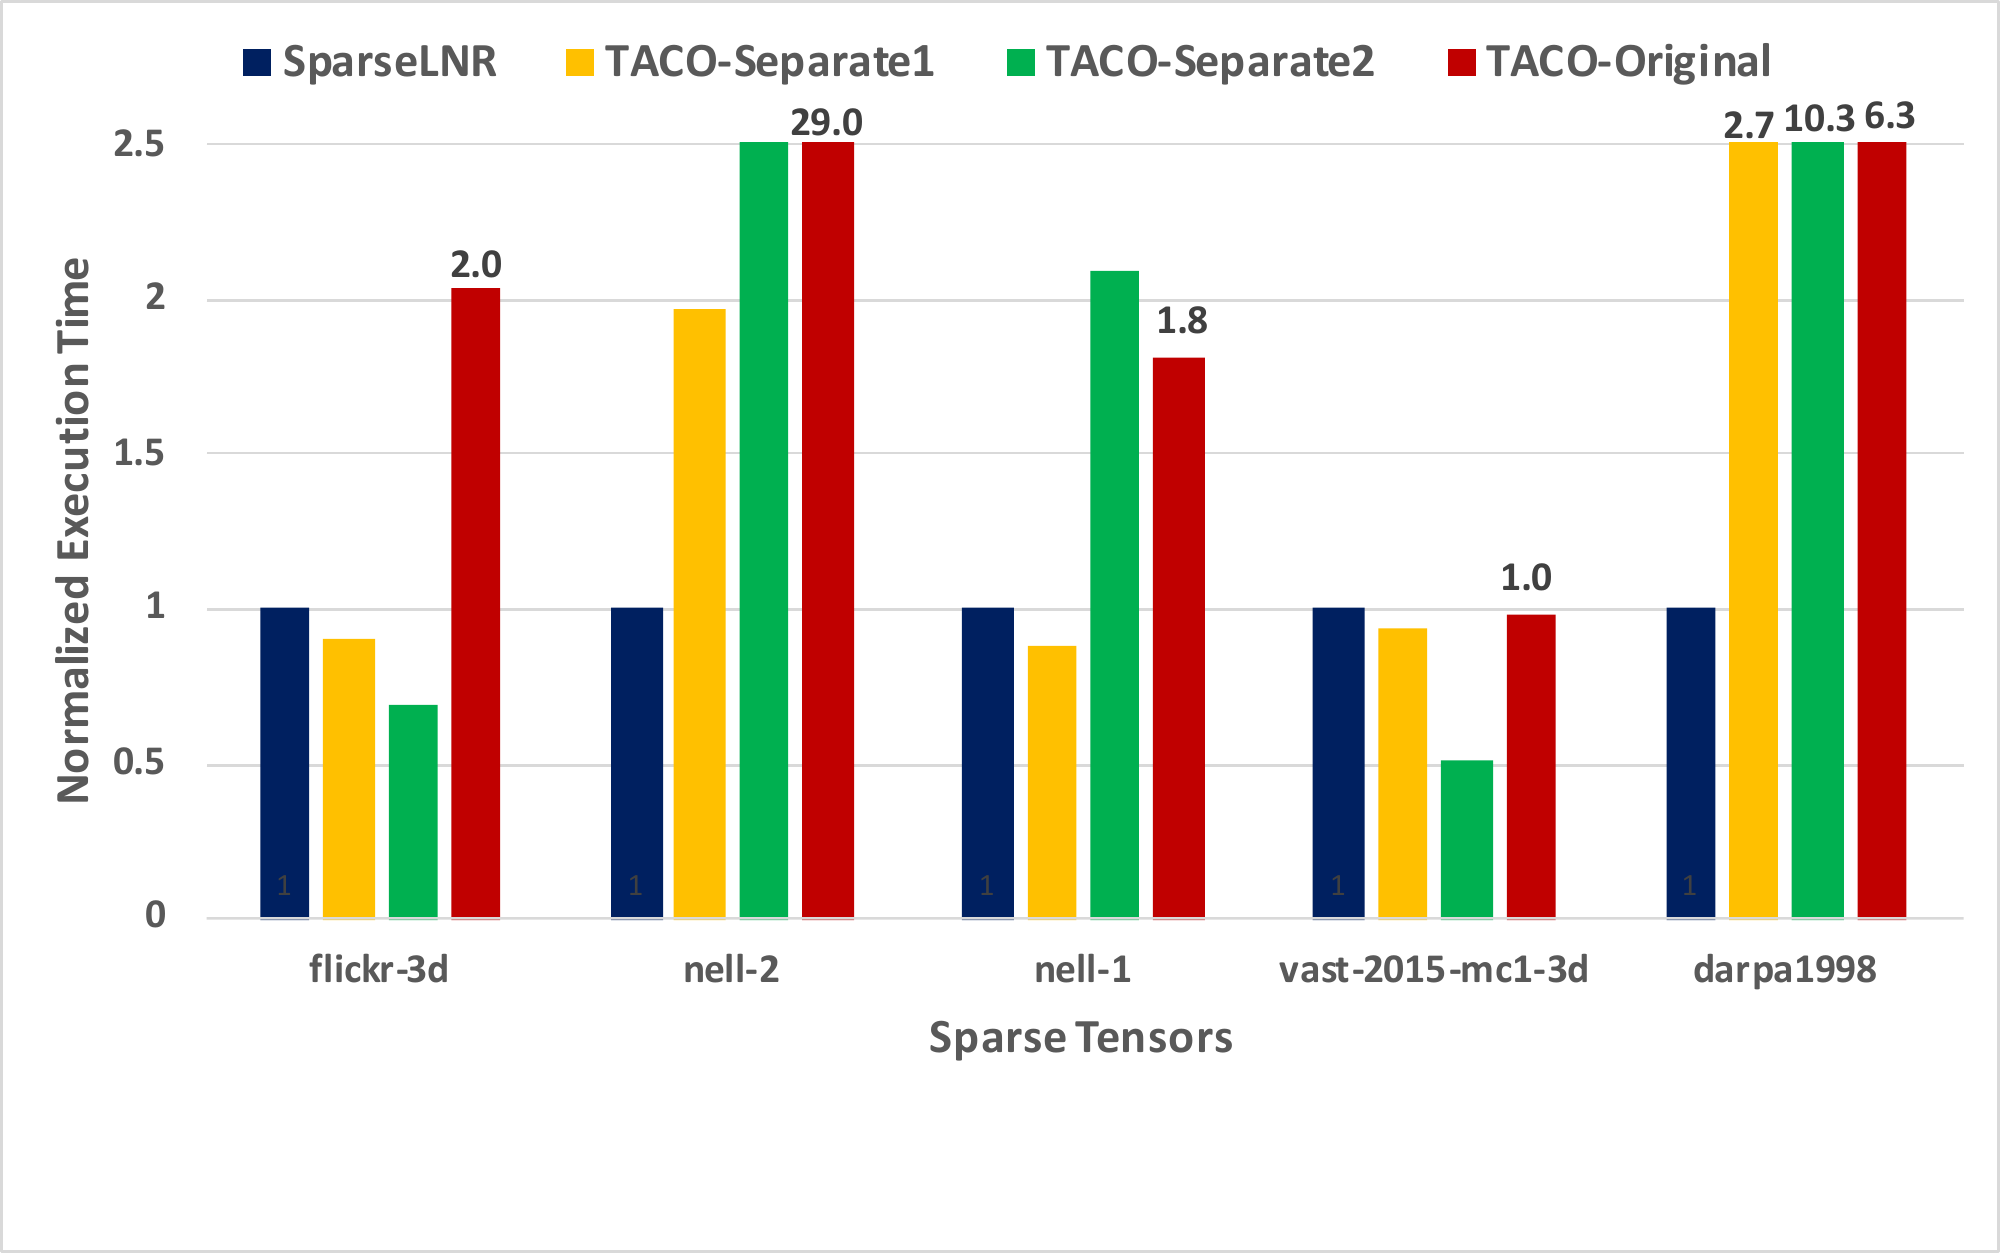}
        \vspace{-10pt}
        \caption{<SpTTM, SpTTM> multi-threads}
        \vspace{-10pt}
        \label{fig:ttm-ttm-multi-thread}
        \Description[sddmm-spmm original iteration graph]{<long description>}
    \end{subfigure}%
    \caption{Performance Comparison with TACO}
    \label{fig:evaluation-of-matrices}
\end{figure*}
